# Supplementary material for: Low-Temperature Kinetic Isotope Effects in CH3OH+H -> CH2OH+H2 Shed Light on the Deuteration of Methanol in Space
Source: arXiv:2009.04308 source file (2020-09-09)
Supplement: Supplementary file 1 [file supporting_info.pdf]

# Supporting information to: Low-Temperature Kinetic Isotope Effects in $CH_3OH + H \rightarrow CH_2OH + H_2$ Shed Light on the Deuteration of Methanol in Space

April M. Cooper and Johannes Kästner*

*Institute for Theoretical Chemistry, University of Stuttgart, Pfaffenwaldring 55, 70569 Stuttgart, Germany*

E-mail: kaestner@theochem.uni-stuttgart.de

Phone: +49-711-685-64473

Table S1: Bimolecular rate constants for R1 with incoming H, obtained from a microcanonical formalism.

| T (K) | Rate Constant ($cm^3 s^{-1}$) |
|---|---|
| 343.1 | $2.604 \cdot 10^{-15}$ |
| 72.4 | $1.561 \cdot 10^{-18}$ |
| 41.3 | $1.325 \cdot 10^{-18}$ |
| 28.4 | $1.467 \cdot 10^{-18}$ |
| 21.7 | $1.759 \cdot 10^{-18}$ |
| 17.6 | $2.174 \cdot 10^{-18}$ |
| 14.7 | $2.694 \cdot 10^{-18}$ |
| 12.8 | $3.268 \cdot 10^{-18}$ |
| 11.2 | $3.936 \cdot 10^{-18}$ |
| 10.0 | $4.660 \cdot 10^{-18}$ |

Table S2: Unimolecular rate constants ($s^{-1}$) for incoming H (R1-R4).

| T (K) | R1 | R2 | R3 | R4 |
|---|---|---|---|---|
| 260 | $1.908 \cdot 10^{7}$ | $1.078 \cdot 10^{7}$ | $4.668 \cdot 10^{6}$ | $1.559 \cdot 10^{5}$ |
| 150 | $4.081 \cdot 10^{5}$ | $2.082 \cdot 10^{5}$ | $8.194 \cdot 10^{4}$ | $5.060 \cdot 10^{2}$ |
| 105 | $7.516 \cdot 10^{4}$ | $3.571 \cdot 10^{4}$ | $1.367 \cdot 10^{4}$ | $4.055 \cdot 10^{1}$ |
| 75 | $2.583 \cdot 10^{4}$ | $1.124 \cdot 10^{4}$ | $4.411 \cdot 10^{3}$ | $9.020 \cdot 10^{0}$ |
| 60 | $1.489 \cdot 10^{4}$ | $6.396 \cdot 10^{3}$ | $2.549 \cdot 10^{3}$ | $4.642 \cdot 10^{0}$ |
| 50 | $1.055 \cdot 10^{4}$ | $4.595 \cdot 10^{3}$ | $1.808 \cdot 10^{3}$ | $3.014 \cdot 10^{0}$ |
| 45 | $9.131 \cdot 10^{3}$ | $4.011 \cdot 10^{3}$ | $1.561 \cdot 10^{3}$ | $2.472 \cdot 10^{0}$ |
| 40 | $8.133 \cdot 10^{3}$ | $3.601 \cdot 10^{3}$ | $1.384 \cdot 10^{3}$ | $2.089 \cdot 10^{0}$ |
| 35 | $7.508 \cdot 10^{3}$ | $3.347 \cdot 10^{3}$ | $1.269 \cdot 10^{3}$ | $1.846 \cdot 10^{0}$ |
| 30 | $7.217 \cdot 10^{3}$ | $3.227 \cdot 10^{3}$ | $1.210 \cdot 10^{3}$ | $1.730 \cdot 10^{0}$ |

Table S3: Unimolecular rate constants ($s^{-1}$) for incoming H (R5-R8).

| T (K) | R5 | R6 | R7 | R8 |
|---|---|---|---|---|
| 260 | $2.693 \cdot 10^{5}$ | $3.558 \cdot 10^{5}$ | $1.837 \cdot 10^{7}$ | $1.904 \cdot 10^{7}$ |
| 150 | $7.632 \cdot 10^{2}$ | $8.921 \cdot 10^{2}$ | $3.865 \cdot 10^{5}$ | $4.067 \cdot 10^{5}$ |
| 105 | $5.736 \cdot 10^{1}$ | $6.392 \cdot 10^{1}$ | $7.061 \cdot 10^{4}$ | $7.495 \cdot 10^{4}$ |
| 75 | $1.192 \cdot 10^{1}$ | $1.314 \cdot 10^{1}$ | $2.416 \cdot 10^{4}$ | $2.581 \cdot 10^{4}$ |
| 60 | $5.860 \cdot 10^{0}$ | $6.568 \cdot 10^{0}$ | $1.390 \cdot 10^{4}$ | $1.490 \cdot 10^{4}$ |
| 50 | $3.782 \cdot 10^{0}$ | $4.265 \cdot 10^{0}$ | $9.822 \cdot 10^{3}$ | $1.056 \cdot 10^{4}$ |
| 45 | $3.120 \cdot 10^{0}$ | $3.499 \cdot 10^{0}$ | $8.491 \cdot 10^{3}$ | $9.146 \cdot 10^{3}$ |
| 40 | $2.657 \cdot 10^{0}$ | $2.949 \cdot 10^{0}$ | $7.560 \cdot 10^{3}$ | $8.151 \cdot 10^{3}$ |
| 35 | $2.366 \cdot 10^{0}$ | $2.591 \cdot 10^{0}$ | $6.975 \cdot 10^{3}$ | $7.525 \cdot 10^{3}$ |
| 30 | $2.231 \cdot 10^{0}$ | $2.407 \cdot 10^{0}$ | $6.691 \cdot 10^{3}$ | $7.235 \cdot 10^{3}$ |

Table S4: Unimolecular rate constants ($s^{-1}$) for incoming D.

| T (K) | R1 | R2 | R3 | R4 | R5 | R6 |
|---|---|---|---|---|---|---|
| 260 | $3.871 \cdot 10^{7}$ | $2.216 \cdot 10^{7}$ | $9.690 \cdot 10^{6}$ | $3.784 \cdot 10^{5}$ | $6.546 \cdot 10^{5}$ | $8.654 \cdot 10^{5}$ |
| 150 | $4.430 \cdot 10^{5}$ | $2.317 \cdot 10^{5}$ | $9.249 \cdot 10^{4}$ | $9.846 \cdot 10^{2}$ | $1.512 \cdot 10^{3}$ | $1.793 \cdot 10^{3}$ |
| 105 | $4.502 \cdot 10^{4}$ | $2.170 \cdot 10^{4}$ | $8.284 \cdot 10^{3}$ | $3.982 \cdot 10^{1}$ | $5.694 \cdot 10^{1}$ | $6.348 \cdot 10^{1}$ |
| 75 | $9.051 \cdot 10^{3}$ | $3.893 \cdot 10^{3}$ | $1.513 \cdot 10^{3}$ | $4.611 \cdot 10^{0}$ | $6.069 \cdot 10^{0}$ | $6.551 \cdot 10^{0}$ |
| 60 | $3.769 \cdot 10^{3}$ | $1.576 \cdot 10^{3}$ | $6.217 \cdot 10^{2}$ | $1.643 \cdot 10^{0}$ | $2.023 \cdot 10^{0}$ | $2.209 \cdot 10^{0}$ |
| 50 | $2.102 \cdot 10^{3}$ | $8.886 \cdot 10^{2}$ | $3.435 \cdot 10^{2}$ | $8.187 \cdot 10^{-1}$ | $9.850 \cdot 10^{-1}$ | $1.084 \cdot 10^{0}$ |
| 45 | $1.611 \cdot 10^{3}$ | $6.862 \cdot 10^{2}$ | $2.606 \cdot 10^{2}$ | $5.823 \cdot 10^{-1}$ | $7.022 \cdot 10^{-1}$ | $7.669 \cdot 10^{-1}$ |
| 40 | $1.270 \cdot 10^{3}$ | $5.455 \cdot 10^{2}$ | $2.032 \cdot 10^{2}$ | $4.253 \cdot 10^{-1}$ | $5.167 \cdot 10^{-1}$ | $5.552 \cdot 10^{-1}$ |
| 35 | $1.041 \cdot 10^{3}$ | $4.503 \cdot 10^{2}$ | $1.645 \cdot 10^{2}$ | $3.255 \cdot 10^{-1}$ | $3.984 \cdot 10^{-1}$ | $4.191 \cdot 10^{-1}$ |
| 30 | $8.966 \cdot 10^{2}$ | $3.903 \cdot 10^{2}$ | $1.400 \cdot 10^{2}$ | $2.655 \cdot 10^{-1}$ | $3.272 \cdot 10^{-1}$ | $3.365 \cdot 10^{-1}$ |
